# Supplementary material for: Multi-layered Safety of Redundant Robot Manipulators via Task-oriented Planning and Control
Source: arXiv:2410.17742 source file (2025-03-30)
Supplement: Supplementary file 1 [file appendix.tex]

\label{appendix}

Hence, Eq. () can be rewritten as
\begin{equation}
    \label{eq:dynamics_2}
    \dot{\bm{\mathcal{P}}} + \bm{\mathcal{H}} = \bm{\tau} + \bm{r} \notag 
\end{equation}

Taking the time derivative of $\hat{\bm{r}}$, and using Eqs. (\ref{eq:dynamics_2}) and (\ref{eq:filter}) can yield
\begin{align}
    \label{eq:usde_dot}
    \hat{\bm{r}} 
    &= \int_{0}^{t} { \dot{\hat{\bm{r}}} } \, ds = \int_{0}^{t} { (\frac{\dot{\bm{\mathcal{P}}} - \dot{\bm{\mathcal{P}}_f}} {k} + \dot{\bm{\mathcal{H}}}_f - \dot{\bm{\tau}}_f }) \, ds \notag \\
    &= \int_{0}^{t} { \frac{1}{k} (\dot{\bm{\mathcal{P}}} 
    - \frac{\bm{\mathcal{P}} - \bm{\mathcal{P}}_f} {k} 
    + \bm{\mathcal{H}} - \bm{\mathcal{H}}_f
    - \bm{\tau} + \bm{\tau}_f) } \, ds \notag \\
    &= \frac{1}{k} \int_{0}^{t} { ( \dot{\bm{\mathcal{P}}} + \bm{\mathcal{H}} - \bm{\tau} - (
    \frac{\bm{\mathcal{P}} - \bm{\mathcal{P}}_f} {k} 
    + \bm{\mathcal{H}}_f - \bm{\tau}_f )) } \, ds \notag \\
    &= \frac{1}{k} \left(\bm{\mathcal{P}} + \int_{0}^{t} {(\bm{\mathcal{H}} - \bm{\tau} - \hat{\bm{r}} ) } \, ds \right) \notag \\
    &= \frac{1}{k} \left( \bm{\mathcal{P}} - \int_{0}^{t} {(\bm{\tau} + \bm{C}^\top \dot{\bm{q}} - \bm{g} + \hat{\bm{r}} ) } \, ds \right) \notag
\end{align}
